# Supplementary material for: Convolutional Dynamic Alignment Networks for Interpretable Classifications
Source: arXiv:2104.00032 source file (2024-01-15)
Supplement: Supplementary file 1 [file 1-supp_main.tex]

\documentclass[final]{cvpr_supp}

%%%%%%%%%%%%%%
%% PACKAGES %%
%%%%%%%%%%%%%%
\usepackage{times}
\usepackage{epsfig}
\usepackage{graphicx}
\usepackage{amsmath}
\usepackage{mathtools}
\usepackage{amssymb}
\usepackage{subcaption}
\usepackage{wrapfig}
\usepackage{multirow}
\usepackage{amsthm}
\usepackage{changepage}

\usepackage{algorithm2e,setspace}
\usepackage[document]{ragged2e}
\usepackage{parskip}
\usepackage{array}
\usepackage{enumitem}       % enumerations

\usepackage{xcolor}
\usepackage[pagebackref=true,breaklinks=true,colorlinks,bookmarks=false]{hyperref}

 % *** Enter the CVPR Paper ID here

%\setcounter{page}{4321} % For final version only

%%%%%%%%%%%%%%
%% COMMANDS %%
%%%%%%%%%%%%%%

 % As a dummy until defined.

\begin{document}
\pagecolor{white}
\input{appendix_content}
\end{document}
