# Supplementary material for: Convolutional Dynamic Alignment Networks for Interpretable Classifications
Source: arXiv:2104.00032 source file (2024-01-15)
Supplement: Supplementary file 2 [file 0.0-packages_and_commands_supp.tex]

%%%%%%%%%%%%%%
%% PACKAGES %%
%%%%%%%%%%%%%%
\usepackage{times}
\usepackage{epsfig}
\usepackage{graphicx}
\usepackage{amsmath}
\usepackage{mathtools}
\usepackage{amssymb}
\usepackage{subcaption}
\usepackage{wrapfig}
\usepackage{multirow}
\usepackage{amsthm}
\usepackage{changepage}

\usepackage{algorithm2e,setspace}
\usepackage[document]{ragged2e}
\usepackage{parskip}
\usepackage{array}
\usepackage{enumitem}       % enumerations

\usepackage{xcolor}
\usepackage[pagebackref=true,breaklinks=true,colorlinks,bookmarks=false]{hyperref}

\def\cvprPaperID{9920} % *** Enter the CVPR Paper ID here
\def\confYear{CVPR 2021}
%\setcounter{page}{4321} % For final version only

%%%%%%%%%%%%%%
%% COMMANDS %%
%%%%%%%%%%%%%%
\newcommand{\colornum}[1]{{\textbf{\color[RGB]{39, 158, 206}#1}}}
\newcommand{\mat}[1]{\MakeUppercase{\mathbf{#1}}}
\renewcommand{\vec}[1]{\MakeLowercase{\mathbf{#1}}}
\newcommand{\tmat}[1]{$\mat{#1}$}
\newcommand{\vmat}[1]{$\vec{#1}$}
\newcommand{\putfig}{} % As a dummy until defined.
\newcommand{\myparagraph}[2][-.5]{\vspace{#1em}\noindent{\bf #2}}

\newcommand{\tbd}[1]{{\color[RGB]{25, 150, 0}TBD: #1}}
